# Supplementary material for: Hierarchical Diffusion Autoencoders and Disentangled Image Manipulation
Source: arXiv:2304.11829 source file (2023-04-25)
Supplement: Supplementary file 2 [file HDAEM_plot.tex]

\begin{figure}[t]
    \centering
    \includegraphics[width=1\linewidth]{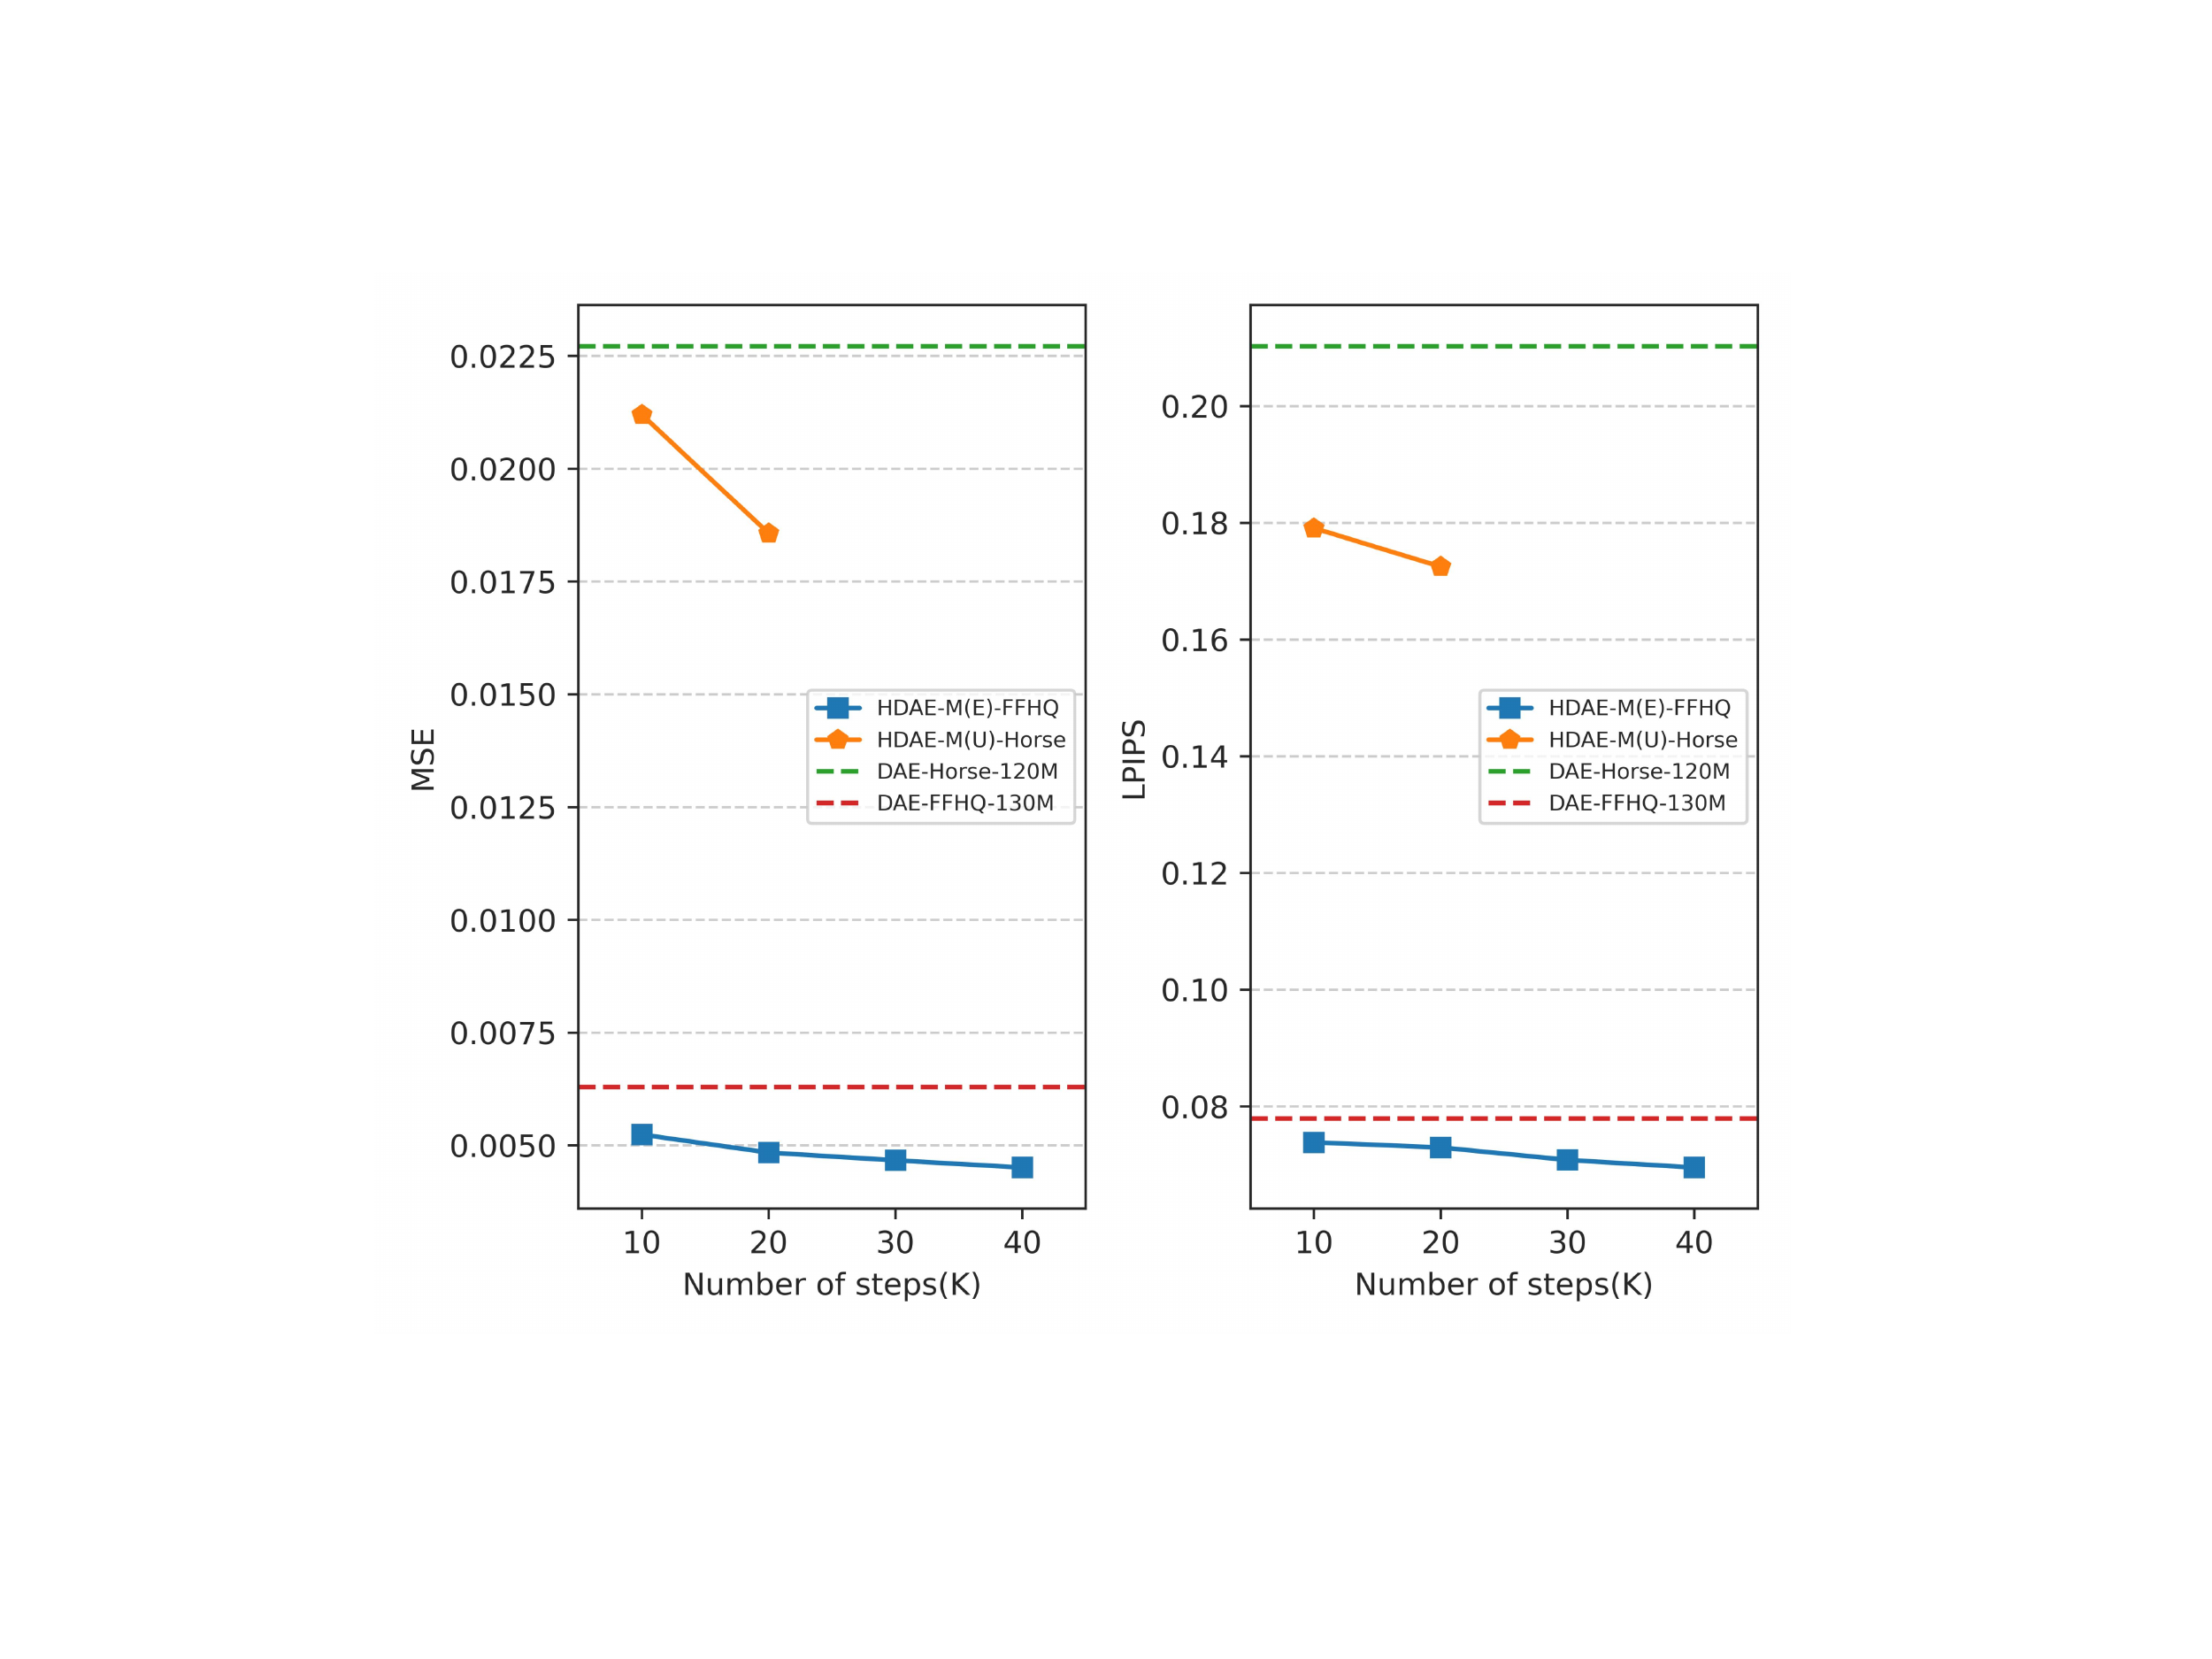}
    \caption{
        \textbf{Image reconstruction results on FFHQ-128 and LSUN Horse-128 for HDAE-M and DAE~\cite{DAE}.} 
        Green lines represent results of DAE trained on LSUN Horse-128 with 120M training images and red lines represent results of DAE trained on FFHQ-128 with 130M training images. 
        HDAE-M(U)-horse was tuned from ``120M'' pretrained checkpoint using HDAE(U) on LSUN Horse-128 and HDAE-M(E)-FFHQ was tuned from ``100M'' pretrained checkpoint using HDAE(E) on FFHQ-128.
    }
    \label{HDAEM}
\end{figure}
