# Supplementary material for: Hierarchical Diffusion Autoencoders and Disentangled Image Manipulation
Source: arXiv:2304.11829 source file (2023-04-25)
Supplement: Supplementary file 3 [file tab_u_gen.tex]

\begin{table}[]
\resizebox{1\linewidth}{!}{
\begin{tabular}{l|c|c}
\toprule[1.2pt]
\textbf{Model}    & \textbf{Setting}                              & \textbf{FID}($\downarrow$)   \\ \midrule[1.2pt]%\hline
DDIM~\cite{DDIM}    & T=20                                 & 12.70 \\ \midrule[1.2pt]%\hline
DAE~\cite{DAE}     & 10 layers, MLP hidden size 2048,T=20 & 10.18 \\ \midrule[1.2pt]%\hline
HDAE(U) & 10 layers, MLP hidden size 4096,T=20 & 14.83 \\
        & 10 layers, MLP hidden size 2048,T=20 & 14.99 \\
        & 10 layers, MLP hidden size 8192,T=20 & 14.99 \\
        & 20 layers, MLP hidden size 4096,T=20 & 15.09 \\
 \bottomrule[1.2pt]
\end{tabular}
}
\caption{
\textbf{Unconditional generation results of DDIM~\cite{DDIM}, DAE~\cite{DAE} and HDAE(U) on the CelebA~\cite{celeba}}}
\label{tab_u_gen_sup}
\end{table}
