# Supplementary material for: Hierarchical Diffusion Autoencoders and Disentangled Image Manipulation
Source: arXiv:2304.11829 source file (2023-04-25)
Supplement: Supplementary file 4 [file tab_user_study.tex]

\begin{table}[t]
\resizebox{1\linewidth}{!}{
\begin{tabular}{l|ccc}
\toprule[1.2pt]
\textbf{Task} & \textbf{HDAE(U) Disentangle}   & \textbf{HDAE(U)} & \textbf{DAE} \\ \midrule[1.2pt]
Image Manipulation  & 69.33\% &  22.28\%  & 8.38\% \\ \bottomrule[1.2pt]
\end{tabular}
}
\caption{
    \textbf{Human perceptual evaluation on image manipulation.} 
    ``HDAE(U) Disentangle'' means disentangled image manipulation with truncated feature using HDAE(U).
}
\label{tab_userstudy_sup}
\end{table}
